# Supplementary material for: ForgeMegakernel: A General Framework for Efficient Auto-Regressive Model Decode Megakernels
Source: arXiv:2609.12379 source file (2026-09-11)
Supplement: Supplementary file 1 [file 09-appendix.tex]

\section{Tuning the engine baselines}
\label{sec:appendix:knobs}

Every ratio in this paper divides by a baseline, so a baseline slower than the
engine can be inflates all of them, which is the one direction the error must not
go.
Both engines were originally measured at their library defaults, and the defaults
are not the fast configuration.

\input{sec/tab-knobs}

\paragraph{What ``latest'' means on this cluster.} The node driver is 550.90.07
(CUDA~12.6), and taken alone it caps the search below either engine's newest
release: vLLM~$\ge$~0.27 and SGLang~$\ge$~0.5.16 need a CUDA-13 torch, which dies
at \code{\_cuda\_init} against a 12.6 driver. The cap is a property of the
\emph{container}, not of the card: an image carrying NVIDIA's
forward-compatibility libraries supplies a 580.95.05 user-mode driver over the
same kernel driver, and a cu130 torch then runs on the same node and the same
card. We therefore report vLLM~0.27.1 and SGLang~0.5.18, both on
torch~2.13.0+cu130. Each engine is installed into a clean virtual environment and
verified by a real CUDA initialisation plus the import the backend actually
makes, because \code{import vllm} is lazy and succeeds on a broken install. Two
caveats we state rather than hide: the two engine columns run under the
forward-compatibility driver while the megakernel and MPK columns run natively,
and a same-engine control across the two containers has not been measured; and an
engine's argument surface moves between releases, so the harness reads the
accepted argument names from the engine and refuses to run rather than silently
drop a knob it cannot set.

\paragraph{Two results worth print.} First, \code{enable\_torch\_compile}
\emph{alone} beats the cumulative ladder: adding the graph-batch knobs on top of
it costs 0.8 points at $b{=}1$ (Table~\ref{tab:knobs}), so the promoted SGLang
configuration is the single knob, not the stack. Second, the engines are not
symmetric where one would most expect them to be. Skipping tokenizer
initialisation \emph{costs} SGLang 4.9\%, while its vLLM mirror, returning token
ids and never detokenising, gains 2.6\% at $b{=}8$. The argument for the
SGLang knob was clean, and it is still wrong; we leave it off.

\paragraph{What the tuning cost us.} Re-measuring all ten checkpoints at the
promoted configuration gains a median 14.6\% for SGLang and 26.8\% for vLLM over
the older baselines, and moves our geometric mean against SGLang from
$1.44\times$ to $1.19\times$ at the kernels as first forged; \S\ref{sec:eval:main}
reports $1.21\times$ because six of those kernels have since been forged further
after first publication. The corroborating evidence
that the new baselines are tuned rather than merely newer is that the two engines
now agree with each other: median SGLang/vLLM latency ratio 0.96 with 34 of 39
configurations inside $\pm$10\%, against 0.81 and 5 of 38 before.

\section{Correctness against exact arithmetic}
\label{sec:appendix:accuracy}

Correctness is scored against an independent float64 forward: the canonical bf16
checkpoint upcast exactly and run with no rounding boundary. Both decoders are
teacher-forced at every position of the same prompts and their next-token top-1
choices compared to the golden's, paired. The reference matters: scored against
\emph{SGLang} rather than the truth, configurations where the unmodified engine
itself drifts read as our failures, and it is 2.0--2.6\% from the golden on
three of the eleven configurations
with a teacher-forced pass.

Over 96--16{,}287 teacher-forced positions per configuration, 9 of the 11 forged
megakernels with such a pass are strictly closer to exact arithmetic than
unmodified SGLang, one ties,
and one (Llama-2-13B-chat) is two positions of 508 below it
(Table~\ref{tab:cells}, \emph{golden}). Every such raw miss is \emph{sub-ulp}:
the reference's own runner-up at a top-two logit gap below one bf16 quantum, a
tie broken by summation order rather than by correctness. Masking off in both
decoders the positions the golden cannot itself separate by at least one bf16 ulp (3--9\%
of positions, symmetric), the megakernel is at zero misses on 10 of those 11 and
no worse than the unmodified engine on all 11, and the same holds across all 14 measured this
way.

\section{The float64 reference for the 13B configuration}
\label{sec:appendix:golden}

Llama-2-13B-chat is the one configuration whose reference was itself in question. 13B
parameters in float64 are 96.9\,GiB and do not fit one card, so the configuration was
first scored against a float32 golden, and it is also the only configuration where
unmodified SGLang reads a perfect $1.0000$. We re-ran it in float64 across two cards.
Every number is identical, to the position: $508/508$ and $506/508$ raw,
$488/488$ both on the decidable subset, and the same 20 undecidable positions.
That is the arithmetically coherent outcome rather than a surprise: float32 and
float64 disagree at ${\sim}10^{-4}$ relative in a 13B forward while one bf16 ulp
is ${\sim}10^{-2}$, so both references lie deep inside the same quantum at every
position, and neither the argmax nor the decidability class can move. The
unmodified engine's perfect score on this configuration is a property of the
configuration, not of the instrument.

\section{Defect taxonomy}
\label{sec:appendix:defects}

\input{sec/tab-defects}

Table~\ref{tab:defects} is the catalogue behind \S\ref{sec:obs:oracle}: every
way a round in this project measured well and was wrong anyway, the instance we
observed, and the countermeasure now in the ladder.

\paragraph{Ladder cost.} The 1{,}770 gate runs, about 1.4 per round, dominate
wall-clock time, and the ladder costs rounds directly: 120 of 146 \rung{M6}, 137
of 165 \rung{M7} and 150 of 218 \rung{M8} runs failed. That is the intended
operating point, since a performance milestone passed on the first try has its
floor set too low. Of the forced checks the most valuable has no tunable at all:
\textsf{poison\_canary} sees a read past the KV write cursor, which every
distribution metric is blind to. Repairing two defects in the width judge took
\eqcite{eq:alpha} from abstaining on half the configurations to deciding all of them, and
immediately exposed five kernels computing the wrong rotary embedding. Review
rounds were 376 of the 1{,}489 and returned 6 failures, a low yield in a class
the gates cannot reach, where one undetected instance invalidates every later
round rather than one.

\section{The cells with no row}
\label{sec:appendix:heldback}

Fourteen cells produced a kernel with no row in
Table~\ref{tab:cells}. \emph{Three are the withdrawn Llama-3.2-1B configurations} of
\S\ref{sec:eval:setup}: two clear every bar, but the checkpoint is untrained.
\emph{Three failed the precision contract at competitive speed}:
\code{qwen3-4b-\allowbreak b4s2048} at 66.2\% MBU, with three accumulation macros
defaulting to a bf16 multiply--add chain no build flag overrode;
\code{qwen3-0.6b} at 41.3\%, with a live
\code{constexpr bool} turning its rounding helper into a real bf16 rounding on
the norm gain, the in-kernel sine/cosine table, every rotation product and the
SiLU; and \code{minicpm4-0.5b}, which rounds its rotary table to bf16 on the
measured path. All three are faster than megakernels we did forge, which is exactly
why the contract, not speed, decides. \emph{Three failed the MBU or parity bars}:
\code{minicpm5-1b} (b1, S1024) at 27.9\% MBU and $0.77\times$ SGLang,
\code{minicpm5-1b-\allowbreak b16s2048} at 16.4\% and $0.42\times$, and
\code{minicpm4-3b-\allowbreak b16s1024} at 36.7\%, below the 40\% floor. All
three ratios are against SGLang~0.5.18 at the promoted configuration, the same
baseline as Table~\ref{tab:cells}.
\emph{One is redundant}: \code{minicpm4-3b-\allowbreak b8s2048} clears every bar
but carries the same ragged-position defect as its withheld $b{=}16$ sibling and
collapses to the same 0.025 on GSM8K. The remaining four are process losses: one
ran on a clock-locked card, two stalled below \rung{M7} (NanBeige4-3B at 32.1\%
and Qwen2.5-3B at 41.6\%), and one cleared \rung{M8} at target tier (70.0\%) but
arrived after the publication pass.

\section{Which kernel serves which request}
\label{sec:appendix:routing}

\SEQBODY
